# Supplementary material for: Learning Decentralized Strategies for a Perimeter Defense Game with Graph Neural Networks
Source: arXiv:2211.01757 source file (2022-09-24)
Supplement: Supplementary file 1 [file 7.Appendix.tex]

\appendix
\section{One-on-one Hemisphere Perimeter Defense}\label{sec:1vs1}
This section details terminologies and basic concepts of 1 vs. 1 hemisphere perimeter defense, which were first introduced in~\citep{lee2020perimeter}. We reiterate them here due to their importance to this body of work.

\subsection{Motivation behind Hemisphere Perimeter Defense}\label{sec:motivation}
\blue{Perimeter defense is a relatively new field of research that has been explored recently. One particular challenge is that the high-dimensional perimeters add spatial and algorithmic complexities for defenders to execute their optimal strategies. Although many previous works considered engagements on a planar game space and derived optimal strategies in 2D motions, the extension towards high-dimensional spaces is unavoidable for practical applications of perimeter defense games in real-world scenarios. For instance, a perimeter of a building that defenders aim to protect can be enclosed by a hemisphere. Since defenders cannot pass through the building, they are employed to move along the surface of the dome, which leads to the “hemisphere perimeter defense game.” The intruder is moving on the base plane of the hemisphere, which implies a constant altitude in moving. The movement of the intruder is constrained to 2D since it is assumed that intruders may want to stay low in altitude to hide from the defenders in the real world.}

\blue{It is worth noting that the hemisphere defense problem is more challenging to solve than a problem where both agents are allowed to freely move in a 3D space. There were previous works in which both defenders and intruders could move in 3-dimensional spaces~\citep{yan2022matching,yan2019construction,yan2020guarding}. In all cases, the authors were able to explicitly derive the optimal solutions even in multi-robot scenarios. Although our problem limits the dynamics of the defenders to the surface of the hemisphere, these constraints make the finding of an optimal solution intractable and challenging.}

\subsection{Optimal Breaching Point}\label{sec:optimal}
Given $\zd$, $\za$, we call $\textit{breaching point}$ as a point on the perimeter at which the intruder tries to reach the target, as shown $B$ in Fig.~\ref{fig:hemisphere}. We call the azimuth angle that forms the breaching point as \textit{breaching angle}, denoted by $\theta$, and call the angle between $(\mf z_A - \mf z_B)$ and the tangent line at $B$ as 

\textit{approach angle}, denoted by $\beta$. It is proved in~\citep{lee2020perimeter} that given the current positions of defender $\mf z_D$ and intruder $\mf z_A$ as point particles, there exists a unique breaching point such that the optimal strategy for both defender and intruder is to move towards it, known as \textit{optimal breaching point}. The breaching angle and approach angle corresponding to the optimal breaching point are known as \textit{optimal breaching angle}, denoted by $\theta^*$, and \textit{optimal approach angle}, denoted by $\beta^*$. As stated in \cite{lee2020perimeter}, although there exists no closed-form solution for $\theta^*$ and $\beta^*$, they can be computed at any time by solving two governing equations:

\begin{equation}
\beta^* =  \cos^{-1}\left(\nu\frac{\cos{\phi_D}\sin{\theta^*}}{\sqrt{1-\cos^2{\phi_D}\cos^2{\theta^*}}}\right)
\label{eq:beta}
\end{equation}
and
\begin{equation}
\theta^* = \psi-\beta^*+\cos^{-1}\left(\frac{\cos\beta^*}{r}\right) \label{eq:theta}
\end{equation}

\subsection{Target Time and Payoff Function}\label{sec:payoff}
We call the \textit{target time} as the time to reach $B$ and define $\tdd$ as the \textit{defender target time}, $\taa$ as the \textit{intruder target time}, and the following as \textit{payoff} function:

\bql
\pp = \tdd -\taa \label{eq:payoff}
\eql   

The defender reaches $B$ faster if $p<0$ and the intruder reaches $B$ faster if $p>0$. Thus, the defender aims to minimize $p$ while the intruder aims to maximize it.

\subsection{Optimal Strategies and Nash Equilibrium  \label{sec:nash}}
It is proven in \cite{lee2020perimeter} that the optimal strategies for both defender and intruder are to move towards the optimal breaching point at their maximum speed at any time. Let $\Omega$ and $\Gamma$ be the continuous $v_D$ and $v_A$ that lead to $B$ so that $\td \triangleq \tdd$ and $\ta \triangleq \taa$, and let $\Omega^*$ and $\Gamma^*$ be the optimal strategies that minimize $\td$ and $\ta$, respectively, then the optimality in the game is given as a Nash equilibrium:
\bql
\pdstar\leq\pdastar\leq\pastar \label{eq:nash}
\eql

\section{Graph Neural Networks} \label{sec:gnn}
% We briefly introduce the concepts of graph operations~\cite{Gama19-Architectures} and GNN \cite{li2019graph}. 
\paragraph{Graph Shift Operation} We consider each defender $i, i\in \mathcal{V}$ has a feature vector $\mathbf{x}_i \in \mathbb{R}^F$, indicating the post-processed information from $D_i$. By collecting the feature vectors $\mathbf{x}_i$ from all defenders, we have the feature matrix for the defender team $\mf D$ as: 
\begin{equation} \label{eqn:featureMatrix}
    \mathbf{X} 
    = \begin{bmatrix}
        \mathbf{x}_1^{\mathsf{T}} \\
        \vdots \\
        \mathbf{x}_N^{\mathsf{T}}
      \end{bmatrix} = [\mathbf{x}^1, \cdots, \mathbf{x}^F] \in \mathbb{R}^{N\times F},
\end{equation}
where $\mathbf{x}^f \in  \mathbb{R}^N, f \in [1, \cdots, F]$ is the collection of the feature $f$ across all defenders; i.e., $\mathbf{x}^f = [\mathbf{x}_1^f, \cdots, \mathbf{x}_N^f]^{\mathsf{T}}$ with $\mathbf{x}_i^f$ denoting the feature $f$ of $D_i, i\in\mathcal{V}$. We conduct \textit{graph shift operation} for each $D_i$ by a linear combination of its neighboring features, i.e., $\sum_{j\in \mathcal{N}_i} \mathbf{x}_j$. Hence, for all defenders $\mf D$ with graph $\mathcal{G}$, the feature matrix $\mathbf{X}$ after the shift operation becomes $\mathbf{S} \mathbf{X}$ with:   
\begin{equation} \label{eqn:graphShift}
    [\mathbf{S} \mathbf{X}]_{if} 
        = \sum_{j = 1}^{N} [\mathbf{S}]_{ij} [\mathbf{X}]_j^f
        = \sum_{j \in \mathcal{N}_{i}}
           s_{ij} \mathbf{x}_j^f, 
\end{equation}
Here, the adjacency matrix $\mathbf{S}$ is called the \emph{Graph Shift Operator} (GSO)~\cite{Gama19-Architectures}. %to \qingbiao{avoid duplicated notation with set rather than $S$ in~\cite{li2019graph, Gama19-Architectures}.}
% and is represented by the adjacency matrix $\mathbf{S}_{t}$ in this paper to define the topology of the distance-based dynamic communication graph. 
% Th neighbors of $v_{i}$ is defined by a set of nodes $v_{j}$, where $\ccalN_{i} = \{v_{j} \in \ccalV : (v_{j},v_{i}) \in \ccalE_{t}\}$. Here, the second equality in eq.~\eqref{eqn:graphShift} holds because $s_{t}^{ij} = 0$ for all $j \notin \ccalN_{i}$.

\paragraph{Graph Convolution} With the shift operation, we define the \textit{graph convolution} by a linear combination of the \textit{shifted features} on graph $\mathcal{G}$ via $K$-hop communication exchanges \cite{Gama19-Architectures,li2019graph}: 
\begin{equation} \label{eqn:graphConvolution}
    \mathcal{H}(\mathbf{X}; \mathbf{S}) = \sum_{k=0}^{K} \mathbf{S}^{k} \mathbf{X} \mathbf{H}_{k},
\end{equation}
where $\mathbf{H}_{k} \in \mathbb{R}^{F \times G}$ represents the coefficients combining $F$ features of the defenders in the shifted feature matrix $\mathbf{S}^{k} \mathbf{X}$, with $F$ and $G$ denoting the input and output dimensions of the graph convolution. Note that, $\mathbf{S}^{k} \mathbf{X} = \mathbf{S}(\mathbf{S}^{k-1} \mathbf{X}) $ is computed by means of $k$ communication exchanges with $1$-hop neighbors. 

\paragraph{Graph Neural Network} Applying a point-wise non-linearity $\sigma: \mathbb{R} \to \mathbb{R}$ as the activation function to the graph convolution (\Cref{eqn:graphConvolution}), we define \textit{graph perception} as: 
\begin{equation} \label{eqn:graphPerception}
    \mathcal{H}(\mathbf{X}; \mathbf{S}) = \sigma(\sum_{k=0}^{K} \mathbf{S}^{k} \mathbf{X} \mathbf{H}_{k}).
\end{equation}

Then, we define a GNN module by cascading $L$ layers of graph perceptions (\Cref{eqn:graphPerception}):
\begin{equation} \label{eqn:convGNN}
    \mathbf{X}^{\ell} = \sigma \big[ \mathcal{H}^{\ell}(\mathbf{X}^{\ell-1};\mathbf{S}) \big] \quad \text{for} \quad \ell = 1,\cdots,L,
\end{equation}
where the output feature of the previous layer $\ell-1$, $\mathbf{X}^{\ell-1} \in \mathbb{R}^{N \times F^{\ell-1}}$, is taken as input to the current layer $\ell$ to generate the output feature of layer $l$, $\mathbf{X}^{\ell}$. Recall that the input to the first layer is $\mathbf{X}^{0} = \mathbf{X}$ (\Cref{eqn:featureMatrix}). 
% the dimensions of the features from the previous layer by each robot $i$ at time $t$. 
% The GSO $\mathbf{S}$ in eq.~\eqref{eqn:convGNN} is the one corresponding to the communication network at time $t$, $\mathbf{S} = \mathbf{S}_{t}$. 
The output feature of the last layer $\mathbf{X}^{L} \in \mathbb{R}^{N \times G}$, obtained via $K$-hop communications, represents the exchanged and fused information of the defender team $\mf D$.

\section{Architecture Details}\label{sec:architecture}
\subsection{Model Architecture}\label{sec:modelArchitecture}
Our model architecture consists of a 2-layer MLP with 16 and 8 hidden layers to generate the post-processed feature vector $\mf x_i$, a 2-layer GNN with 32 and 128 hidden layers to exchange the collected information from defenders, and a single-layer MLP to produce an assignment likelihood $\mc L$. The layers in MLP and GNN are followed by ReLU.

\subsection{Perception Details}\label{sec:perceptionDetail}
\blue{The defenders' horizontal field of view $FOV$ is chosen as $\pi$ assuming a fisheye-type camera. The number of input features $\mathit{N}_A^f$ and $\mathit{N}_D^f$ is selected as the fixed number of closest detected and neighboring agents, respectively. Although a defender can detect any number of intruders within the sensing range, a fixed number of detections is selected so that the system is scalable. In a decentralized setting, a defender should be able to decide the action based on its local perception. We experimentally chose the fixed number as 10 since an expert algorithm (i.e., maximum matching) would always assign a defender to a robot among the 10 closest intruders. We also promoted communication with a fixed number of closest defenders to make the system scalable. The selected number was 3 since communicating with many other robots would allow every defender to have full information of the environment (i.e., centralized) and 3 is the minimum number that the robots can collect information in every direction if we assume robots are scattered. If there are fewer than 10 detected intruders or 3 neighboring defenders, we hand over dummy values to fill up the perception input matrix. It is important to keep the input features constant since neural networks cannot handle varying feature sizes.}

\subsection{Graph Neural Networks Details}\label{sec:graphDetail}
In implementing graph neural networks, we construct a 1-hop connectivity graph by connecting defenders within communication range $r_c=1$. Given that the default radius is $R=1$, we foresee that three neighboring agents within 1-hop would provide a wide sensing region for the defenders. Accordingly, we assume that communications occur in real-time with $N_D^f=3$. Each defender gathers information as input features that consist of $N_A^f=10$ closest intruder positions and $N_D^f=3$ closest defender positions. The used parameters are summarized in~\Cref{tab:3}.

%%%%%%%%%%%%%%%%%%%%     Table 3     %%%%%%%%%%%%%%%%%%%%%     
\begin{table}[ht]
\begin{center}
\begin{tabular}{c | c c}
\hline
Parameter name & Symbol & Value\\
\hline
Capturing distance & $\epsilon$ & 0.02\\
Field of view & $FOV$ & $\pi$ \\
Number of intruder features & $\mathit{N}_A^f$ & 10\\
Number of defender features & $\mathit{N}_D^f$ & 3\\
Communication range & $r_c$ & 1\\
Default team size & $N_{def}$ & 10 \\
\hline
\end{tabular}
\end{center}
\caption{Parameter setup} 
\label{tab:3}
\end{table}
%%%%%%%%%%%%%%%%%%%%%%%%%%%%%%%%%%%%%%%%%%%%%%%%%%%%%%%%%% 

\section{Implementation Details}\label{sec:implementation}
The experiments are conducted using a 12-core 3.50GHz i9-9920X CPU and an Nvidia GeForce RTX 2080 Ti GPU. We implement the proposed networks using PyTorch v1.10.1~\citep{paszke2019pytorch} accelerated with Cuda v10.2 APIs. We use the Adam optimizer with a momentum of 0.5. The learning rate is scheduled to decay from $5\times10^{-3}$ to $10^{-6}$ within 1500 epochs with batch size 64, using cosine annealing. We choose these hyperparameters for the best performance.

\section{Performance Analysis}\label{sec:training}

\begin{figure}[!h]
    \centering
    \includegraphics[width=0.5\textwidth]{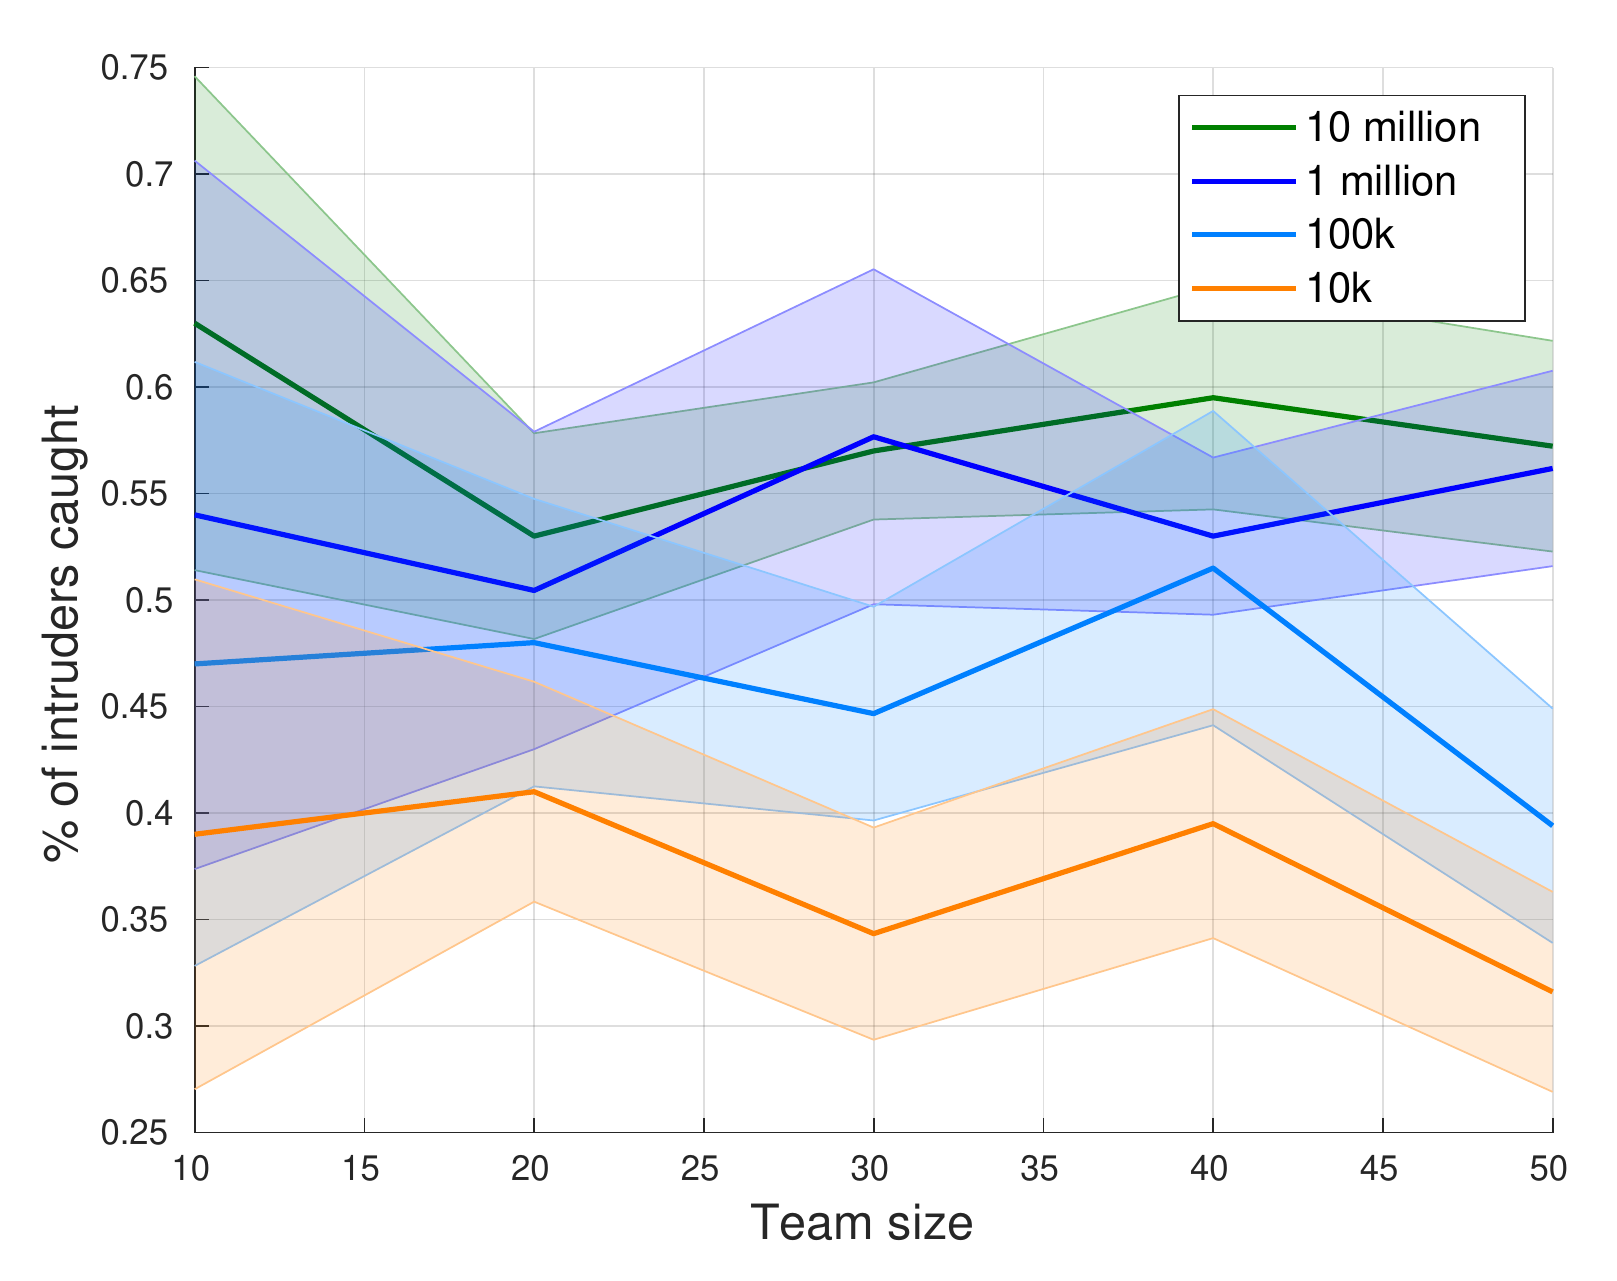}
    \caption{\blue{Sample efficiency with a different number of expert demonstrations.}}
    \label{fig:training}
\end{figure}

\blue{To analyze the algorithm performance, we have trained our GNN-based architecture with a different number of expert demonstrations (e.g., 10 million, 1 million, 100k, and 10k). The percentage of intruders caught (average and standard deviation over 10 trials) on team size $10 \leq N \leq 50$ are shown in~\Cref{fig:training}. The plot validates that our proposed network learns better with more demonstrations.}

\section{Permutation Equivalence}\label{sec:ordering}

\begin{figure}[!h]
    \centering
    \includegraphics[width=1\textwidth]{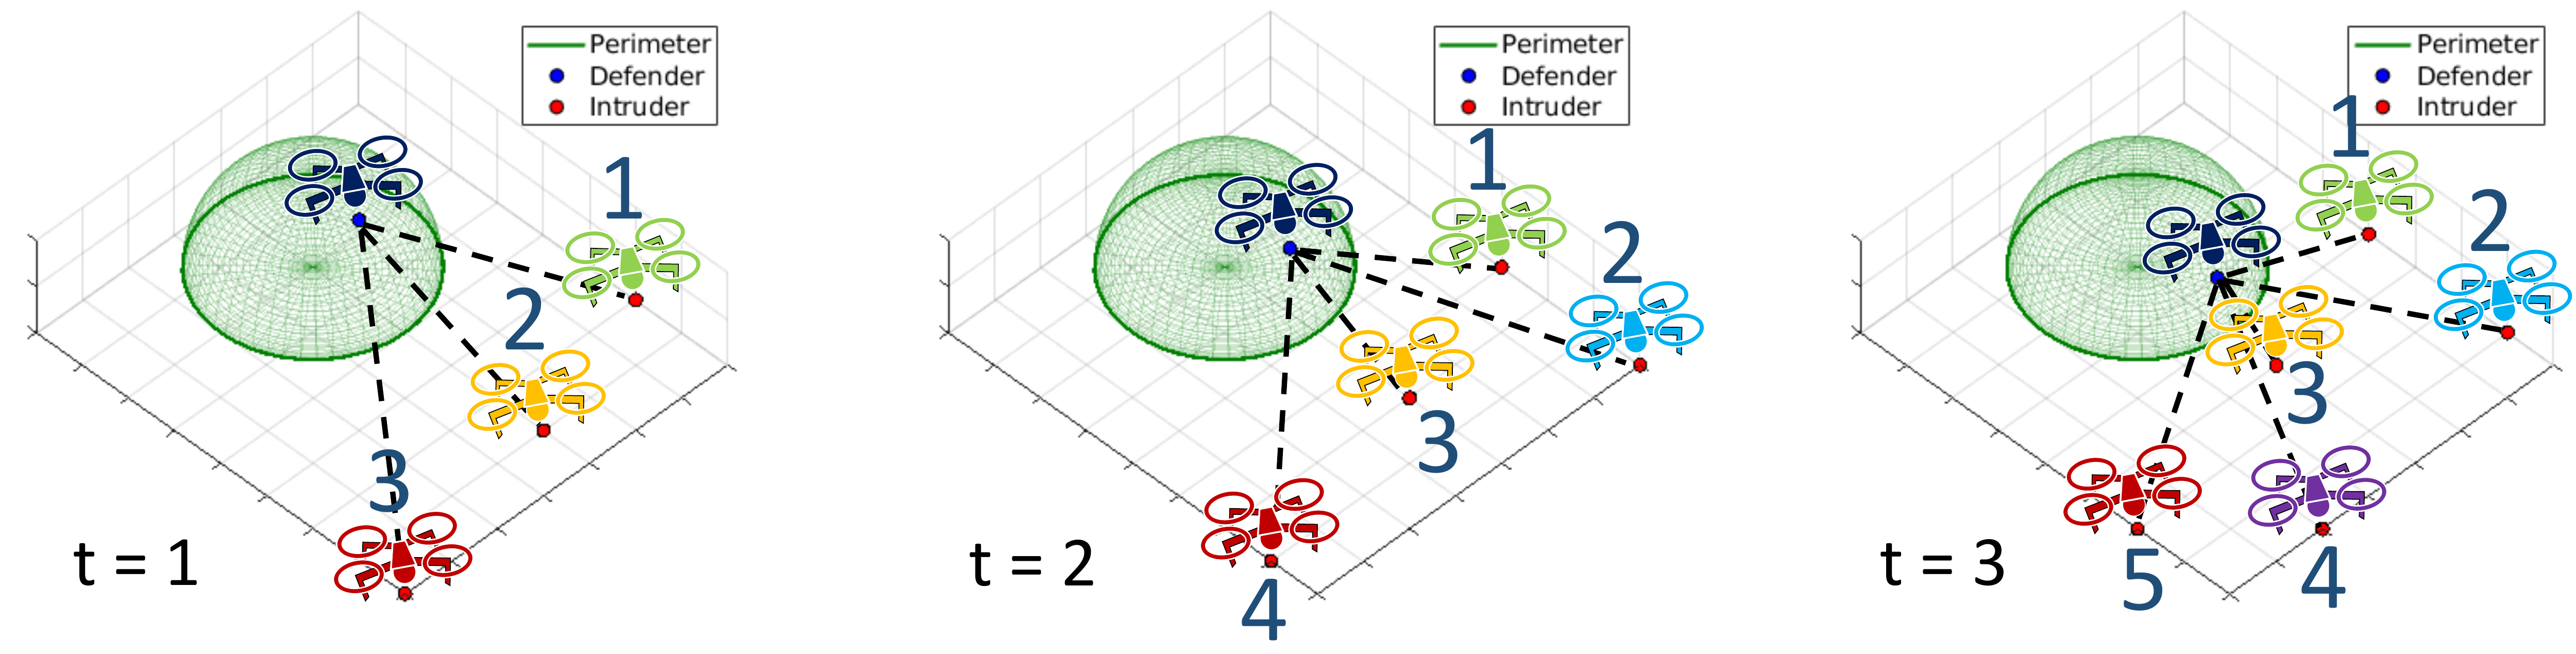}
    \caption{\blue{Instance of perimeter defense game at different time stamps. The plots focus on a single defender and its local perceptions.}}
    \label{fig:ordering}
\end{figure}

\blue{It is worth noting that our proposed GNN-based learning approach is scalable due to permutation equivalence. This means that given a decentralized defender, it should be able to decide the action based on local perceptions that consist of an arbitrary number of unnumbered intruders. An instance of a perimeter defense game is illustrated to show this property in~\Cref{fig:ordering}. The plots focus on a single defender and intruders are gradually approaching the perimeter as time passes by. The same intruders are colored in the same color across different time stamps. Notice that a new light-blue intruder enters into the field of view of the defender at $t=2$, and a purple intruder begins to appear at $t=3$. Although an arbitrary number of intruders are detected at each time, our system gives IDs to intruders shown as blue numbers in~\Cref{fig:ordering}. We number them clockwise but could have done differently in any permutation (e.g., counterclockwise) because graph neural networks perform label-independent processing. The reason for the numbering is to specify which intruders would be matched with which defenders from the network outputs. Without loss of generality, we assign the IDs clockwise but we note that these IDs are arbitrary since the IDs can change at different stamps. For instance, the yellow intruder ID is 2 at $t=1$ but becomes 3 at $t=2,3$. Similarly, the red intruder ID is 3 at $t=1$ but changes to 4 at $t=2$ and 5 at $t=3$. In this way, we accommodate an arbitrary amount of intruders and thus our system is permutation equivalent.}
